# Supplementary material for: Efficient Calculation of NMR Shielding Constants Using Composite Method Approximations and Locally Dense Basis Sets
Source: arXiv:2209.04578 ancillary file (2022-11-12)
Supplement: Supplementary file 1 [file SI.pdf]

# Supporting Information:

## Efficient Calculation of NMR Shielding Constant Using Composite Method Approximations and Locally Dense Basis Sets

Jiashu Liang,<sup>†,¶</sup> Zhe Wang,<sup>†,¶</sup> Jie Li,<sup>†</sup> Jonathan Wong,<sup>†</sup> Xiao Liu,<sup>†</sup> Brad Ganoe,<sup>†</sup>  
Teresa Head-Gordon,<sup>†</sup> and Martin Head-Gordon<sup>\*,†,‡</sup>

<sup>†</sup> *Kenneth S. Pitzer Center for Theoretical Chemistry, Department of Chemistry,  
University of California at Berkeley, Berkeley, CA 94720, USA*

<sup>‡</sup> *Chemical Sciences Division, Lawrence Berkeley National Laboratory, Berkeley, CA  
94720, USA*

<sup>¶</sup> *These authors contributed equally to this work.*

E-mail: mhg@cchem.berkeley.edu

## 1 The method to partition molecules by functional groups

As shown in Figure S1, we can divide molecules into groups based on the non-hydrogen atoms or functional groups. While the first scheme is easy to implement, the second is nontrivial.

Firstly, the xyz2mol code<sup>S1</sup> is employed to convert the molecule geometry in the xyz file to an sdf file, which contains the bonding information of each structure. Then the

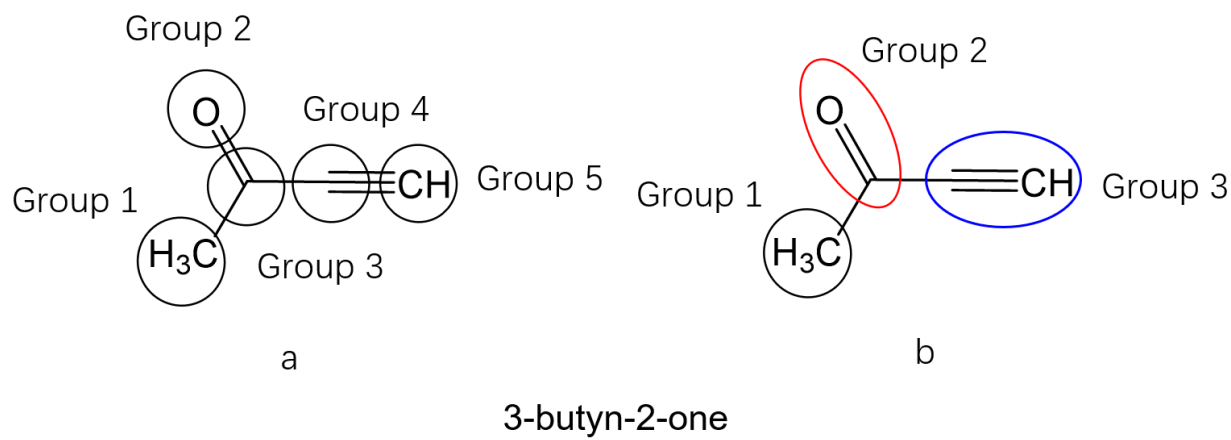

**Figure S1:** Different partitioning methods for LDBS selected for this work, including (a) by non-hydrogen atoms and the bonded hydrogen atoms, and (b) by functional groups

RDKit package<sup>S2</sup> and SMARTS strings<sup>S3</sup> in Table S1 are used to determine typical chemical functional groups according to the sdf file. Once all functional groups have been identified, we designate each group as the target group individually and then define the nearest-neighbor groups and more distant groups according to bonding information. In the case of 3-butyne-2-one (Figure S1), if the target group is alkynyl (blue circle), then carbonyl (red circle) will be the nearest-neighbor group while methyl (black circle) will be the more distant group.

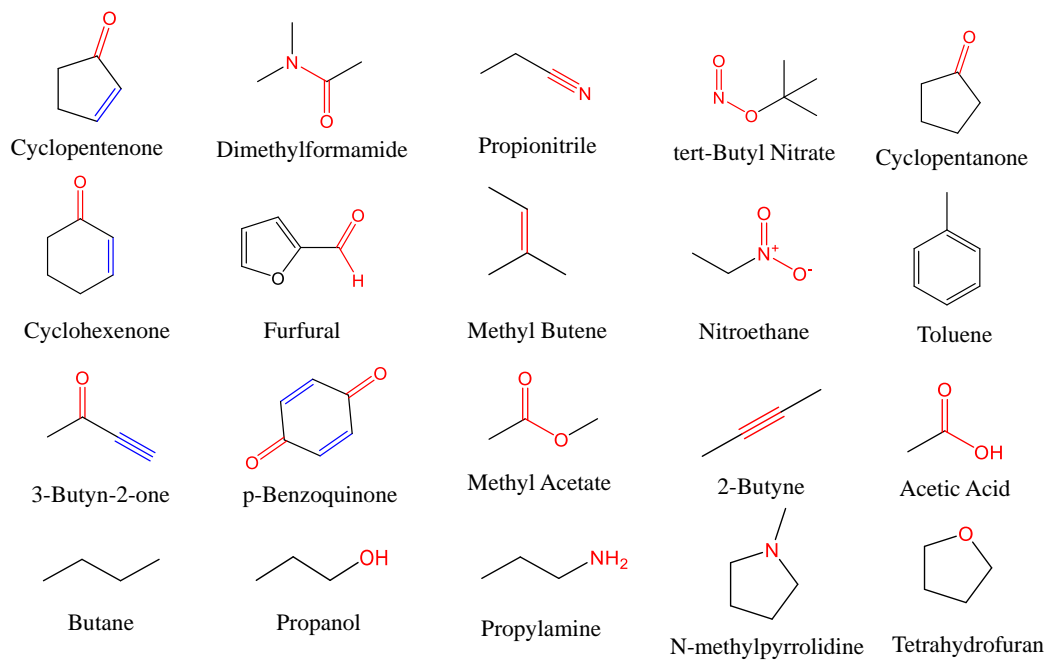

**Figure S2:** Structures of the M20 data set.

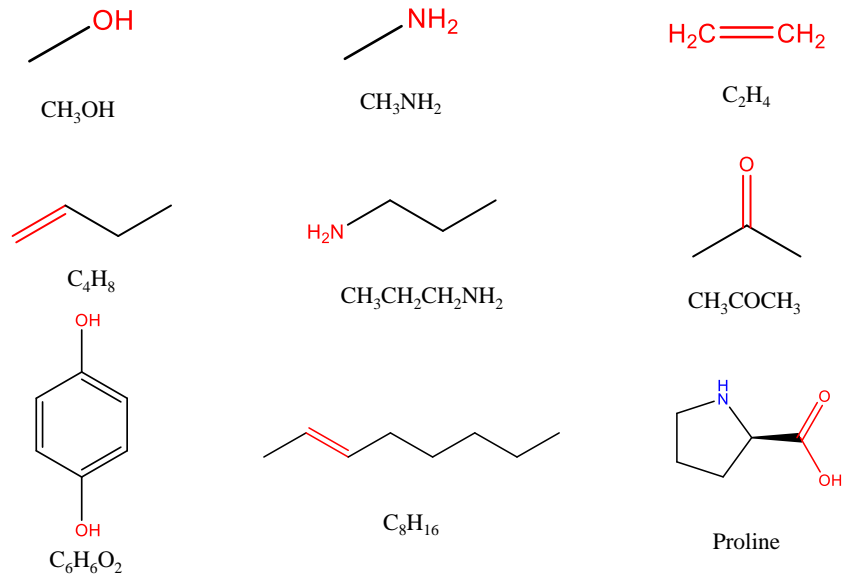

**Figure S3:** Structures of the time evaluation data set.

**Table S1:** SMARTS used in functional group identification in this work. Only functional groups containing no more than three non-hydrogen atoms except nitrate are identified to take full advantage of LDBS.

| SMARTS           |
|------------------|
| [O-][N+](=O)[O-] |
| [C]=[C]=[O]      |
| [O]=[C]=[O]      |
| [C]=[N+]=[N-]    |
| [N-][N+]#[N]     |
| [C]=[C]=[C]      |
| [N]=[C]=[O]      |
| [O]=[C]=[S]      |
| [N+](=O)[O-]     |
| [C](=O)[O]       |
| [C](=O)[N]       |
| [O][N]=[O]       |
| [C]=[O]          |
| [N]#[N]          |
| [N]=[N]          |
| [N]=[O]          |
| [C]#[N]          |
| [C]#[P]          |
| [P]=[O]          |
| [P]#[N]          |
| [P]=[N]          |
| [C]#[C]          |
| [C;v4]=[N]       |
| [C]=[C]          |

## 2 Supplemental figures for main paper

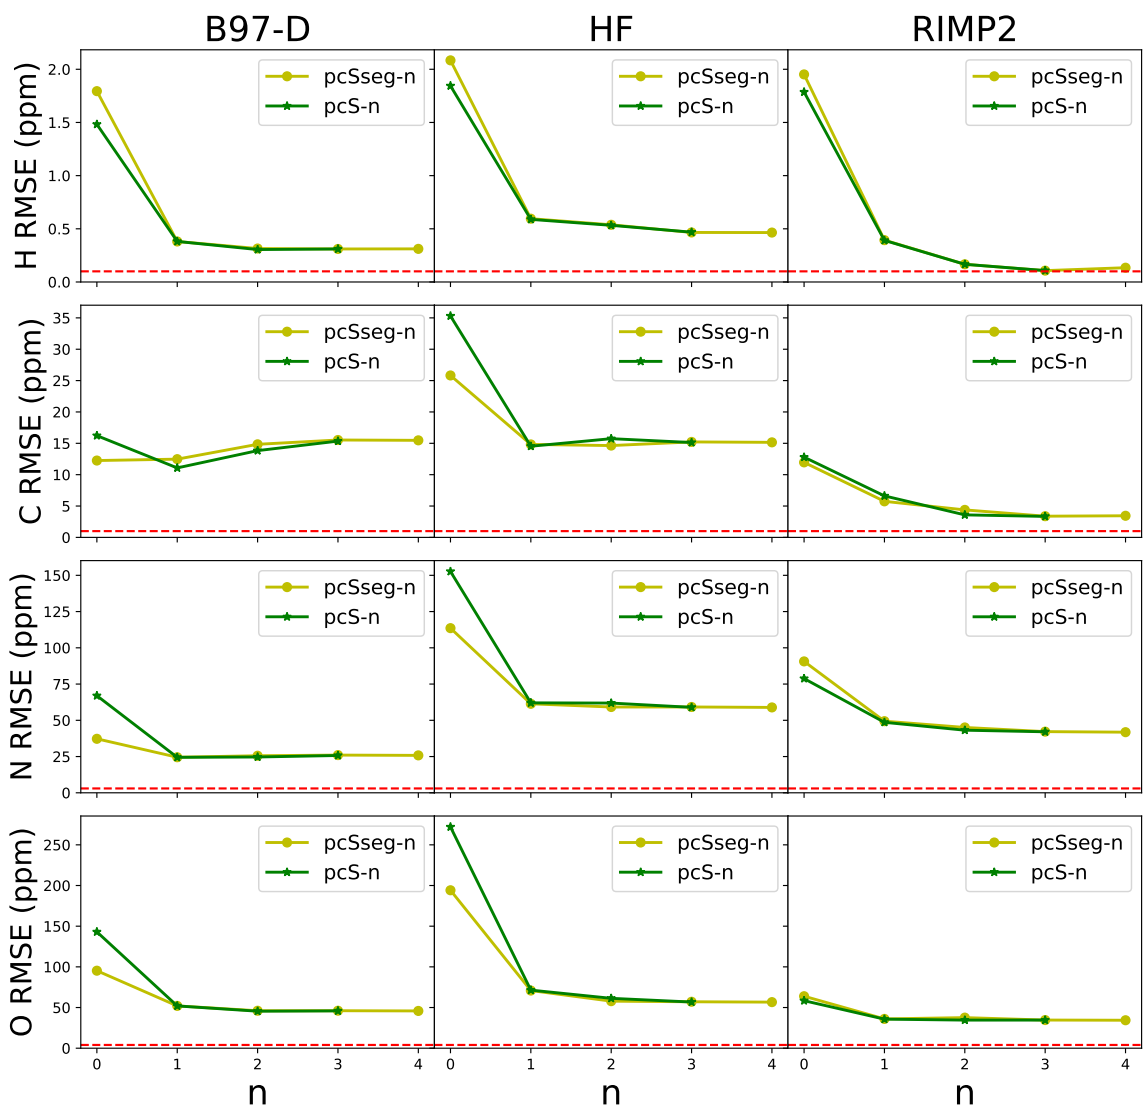

**Figure S4:** Comparison of the RMSEs (in ppm) of pcS-n and pcSseg-n series for B97-D, HF, and RIMP2 with respect to CCSD(T)/pcSseg-4 on H, C, O, and N nuclei. The red horizontal lines indicate an error of 0.1 ppm for H nuclei, 1 ppm for C, 3 ppm for N, and 4 ppm for O.

## References

- (S1) Kim, Y.; Kim, W. Y. Universal structure conversion method for organic molecules: from atomic connectivity to three-dimensional geometry. *Bull. Korean Chem. Soc.* **2015**, *36*,

1769–1777.

(S2) RDKit: open-source cheminformatics. <http://www.rdkit.org>, 2022.

(S3) Daylight Chemical Information Systems, Inc. <https://www.daylight.com/dayhtml/doc/theory/theory.smarts.html>, 2022.
